# Supplementary material for: Nine tips for ecologists using machine learning
Source: arXiv:2305.10472 source file (2023-05-26)
Supplement: Supplementary file 1 [file appendix.tex]

\appendix

\section*{Appendix A. Lynx data analysis}\label{appendixA}

\lstinputlisting[language=R]{appendix_lynx.R}

%\subsection*{References}\label{appendixB:Ref}
%\noindent Chawla, N. V., Bowyer, K. W., Hall, L. O., and Kegelmeyer, W. P. (2002). SMOTE: synthetic minority over-sampling technique. Journal of artificial intelligence research, 16, 321-357.\\
%
%\noindent Lunardon N., Menardi G., and Torelli N. (2014). ROSE: a Package for Binary Imbalanced Learning. R Journal, 6(1), 82-92.\\
%
%\noindent R Core Team (2022). R: A language and environment for statistical computing. R Foundation for Statistical Computing, Vienna, Austria. URL https://www.R-project.org/.\\
%
%\noindent Siriseriwan W. (2019). smotefamily: A Collection of Oversampling Techniques for Class Imbalance Problem Based on SMOTE. R package version 1.3.1. https://CRAN.R-project.org/package=smotefamily\\
%
%\noindent Wright M. and Ziegler A. (2017). ranger: A Fast Implementation of Random Forests for High Dimensional Data in C++ and R. Journal of Statistical Software, 77(1), 1-17. doi:10.18637/jss.v077.i01\\

\section*{Appendix B. Insight into model’s predictions}\label{appendixB}

\lstinputlisting[language=R]{appendix_interpretability.R}

%\subsection*{References}\label{appendixC:Ref}
%Allaire JJ and Chollet F. (2022). keras: R Interface to 'Keras'. R package version 2.8.0. https://CRAN.R-project.org/package=keras\\
%
%\noindent Breiman L: Random forests. J Mach Learn 2001, 45: 5–32. 10.1023/A:1010933404324\\
%
%\noindent R Core Team (2022). R: A language and environment for statistical computing. R Foundation for Statistical Computing, Vienna, Austria. URL https://www.R-project.org/.\\
%
%\noindent Ribeiro, M. T., Singh, S., and Guestrin, C. (2016). " Why should i trust you?" Explaining the predictions of any classifier. In Proceedings of the 22nd ACM SIGKDD international conference on knowledge discovery and data mining (pp. 1135-1144).\\
%
%\noindent Wright M. and Ziegler A. (2017). ranger: A Fast Implementation of Random Forests for High Dimensional Data in C++ and R. Journal of Statistical Software, 77(1), 1-17. doi:10.18637/jss.v077.i01\\
%
%\noindent Zurell, D., Zimmermann, N. E., Gross, H., Baltensweiler, A., Sattler, T., and Wüest, R. O. (2020). Testing species assemblage predictions from stacked and joint species distribution models. Journal of Biogeography, 47(1), 101-113.\\\setcounter{table}{0}
%\renewcommand{\thetable}{A\arabic{table}}

\section*{Appendix C. Flagging label errors in vegetation survey (Box 1)}\label{appendixC}

\lstinputlisting[language=R]{appendix_labelerrors.R}
